# Supplementary material for: Measurement of the multiplicity dependence of $\mit\Upsilon$ production ratios in $pp$ collisions at $\sqrt{s}=13$ TeV
Source: arXiv:2501.12611 source file (2025-05-16)
Supplement: Supplementary file 2 [file appendix.tex]

\section*{Appendices}

\appendix
